# Supplementary material for: A high numerical aperture (NA = 0.92) objective lens for imaging and addressing of cold atoms
Source: arXiv:1611.02159 ancillary file (2016-11-04)
Supplement: Supplementary file 1 [file SupplementaryMaterial.pdf]

# A high numerical aperture (NA = 0.92) objective lens for imaging and addressing of cold atoms: supplementary material

**Carsten Robens[1,*], Stefan Brakhane[1], Wolfgang Alt[1], Felix Kleißler[1], Dieter Meschede[1], Geol Moon[1], Gautam Ramola[1], and Andrea Alberti[1]**

[1] *Institut für Angewandte Physik, Universität Bonn, Wegelerstr. 8, D-53115 Bonn, Germany*
[*] *Corresponding author: robens@iap.uni-bonn.de*

*Compiled November 4, 2016*

**This document provides supplementary information to "A high numerical aperture (NA = 0.92) objective lens for imaging and addressing of cold atoms."**

We present here a description of the effects of the lens apodization (Sec. 1) and of the polar emission profile from the SNOM fiber tip (Sec. 2) on the point spread function (PSF). Both effects require a modification of the pupil function $P$ in Eq. (1) of the main text. In Sec. 3, we provide the details of our objective lens design.

## 1. APODIZATION FUNCTION FOR HIGH NA OBJECTIVE LENSES

Even for a highly corrected objective lens, the image of a point-like isotropic emitter does not result in a collimated beam with a homogeneous intensity distribution [1, 2]. The inhomogeneity becomes especially noticeable for large numerical apertures (NAs). The intensity distribution of the collimated beam depends on the so-called apodization. In the lens design process, one can render the objective lens less sensitive to certain aberrations (stigmatic imaging). The choice of which aberrations to compensate determines the corresponding apodization condition. One example is the so-called Abbe's sine apodization condition, where the objective lens is in first order insensitive to comatic aberration over the field of view [3]. Conceptually, an ideal lens fulfilling Abbe's sine condition can be described by a spherical principal plane, as shown in Fig. 1(a). The resulting apodization function is given by:

$$A_{\text{sine}}(x,y) = \frac{1}{\left(1 - \frac{x^2+y^2}{f_{\text{eff}}^2}\right)^{1/2}}\,, \qquad \textbf{(1)}$$

where we used Abbe's sine condition $f_{\text{eff}} \sin(\theta) = \sqrt{x^2+y^2}$. Since our objective lens fulfills this condition, the intensity of the collimated output beam increases radially from the center towards the edge, see Fig. 1(b). The image of the point source at infinity would deviate from the Airy disk. Specifically, the intensity distribution is slightly narrower, since the apodization increases the weight of the collimated beam's outer part, which is illustrated in Fig. 1(c) for our high NA objective lens. Quantitatively, this effect can be incorporated into the pupil function $P(x,y)$ in Eq. (1) of the main text:

$$P(x,y) = \sqrt{A_{\text{sine}}(x,y)}\,. \qquad \textbf{(2)}$$

## 2. EMISSION PROFILE OF THE SNOM FIBER TIP

An ideal isotropic point source is characterized by an emitted intensity distribution that is invariant in the polar coordinate—the angle $\theta$ spanning the tip axis and the detector direction. Obermüller et al. [4, 5] showed that the light emission from a SNOM fiber tip for emission angles below 10° can be safely considered isotropic. Furthermore, their measurements reveal that the polar intensity distributions for lager emission angles can be well approximated by a Gaussian function for angles below 90°, the width of which in general depends on the light polarization. In the case of a linear polarization the width of the Gaussian distribution parallel to the dipole axis is

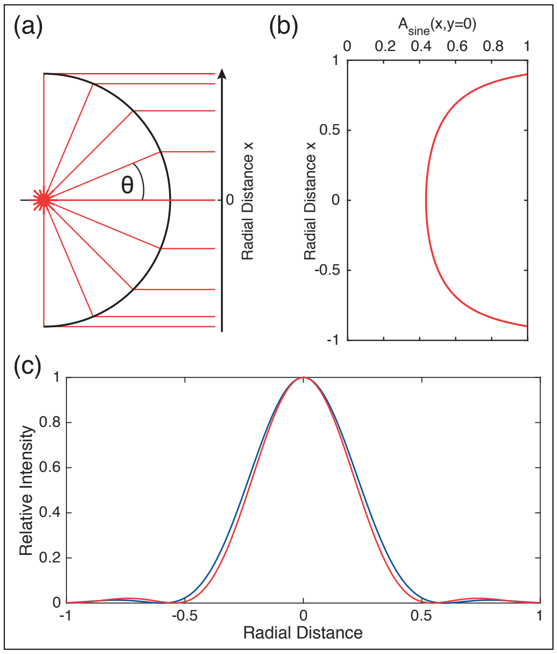


**Fig. 1.** **(a)-(b)** Cut-through illustration of the apodization arising from our high NA objective lens system. Apodization occurs when collimating an isotropic radiation source with a high NA lens, which leads to an inhomogeneous beam profile in the radial direction, as shown here for Abbe's sine condition. **(c)** Point spread functions for an NA = 0.92 objective lens with the apodization effect (red) and without (blue). The apodization leads to a narrower PSF.

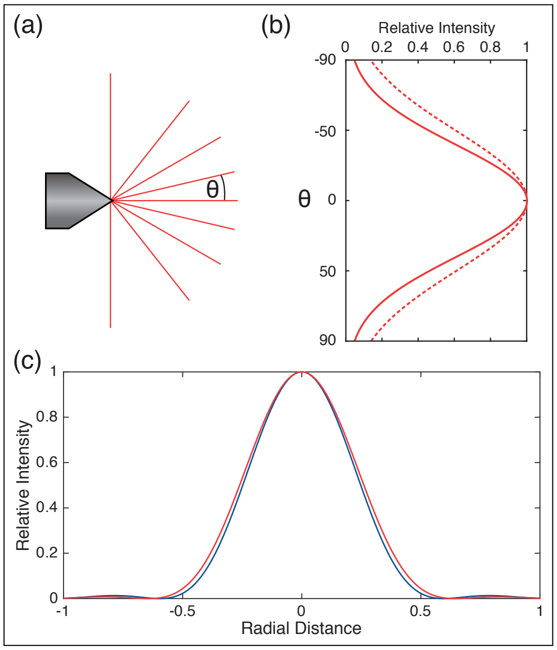


**Fig. 2.** **(a)-(b)** Cut-through illustration of the Gaussian distributed radial emission profile from a SNOM fiber tip. The solid red line represents a distribution with a RMS of $\sigma_{\parallel} = 50°$ and the dashed red line represents a distribution with RMS of $\sigma_{\perp} = 65°$, respectively. **(c)** The red line represents a cut through the PSF parallel to the dipole axis of a NA $= 0.92$ objective lens, whereas the blue line represents a cut through the PSF perpendicular to the dipole axis. The blue curve is visually identical to an ideal Airy disk pattern, whereas the width of the red line is slightly broadened.

narrower than the width in the perpendicular direction. For our SNOM fiber tip ($\varnothing = 200\,\text{nm}$) this amounts to a RMS width of $\sigma_{\parallel} \approx 50°$ and $\sigma_{\perp} \approx 65°$, respectively. The Gaussian distributed emission results in an opposite effect compared to the apodization function: the intensity of the collimated output beam decreases radially from the center towards the edge, see Fig. 2(a). Hence, the image of a point source at infinity is broader than the ideal Airy disk (see Fig. 2(b)). This broadening is illustrated by the red solid line in Fig. 2(c), which shows a cut through the PSF for an axis parallel to the linear polarization. The curve for the perpendicular axis is not shown since deviations from the blue curve of an ideal Airy disk cannot be visually distinguished in the figure. A linear polarization therefore leads to a slightly asymmetric PSF. However, we recover a radially symmetric PSF in our measurements by injecting a circular polarization into the SNOM fiber [6], which effectively averages the two distributions.

Similar to the case of the apodization function mentioned above, we can incorporate this effect by further modifying the pupil function in Eq. (1) of the main text as:

$$P(x,y) = \sqrt{A_{\text{sine}}(x,y)\, f_{\text{Gauss}}(x,y;\sigma_{\parallel},\sigma_{\perp})}\,, \qquad \textbf{(3)}$$

where $f_{\text{Gauss}}$ is a two-dimensional Gaussian distribution with the RMS widths $\sigma_{\parallel}$ and $\sigma_{\perp}$.

## 3. LENS DESIGN DETAILS

(a)

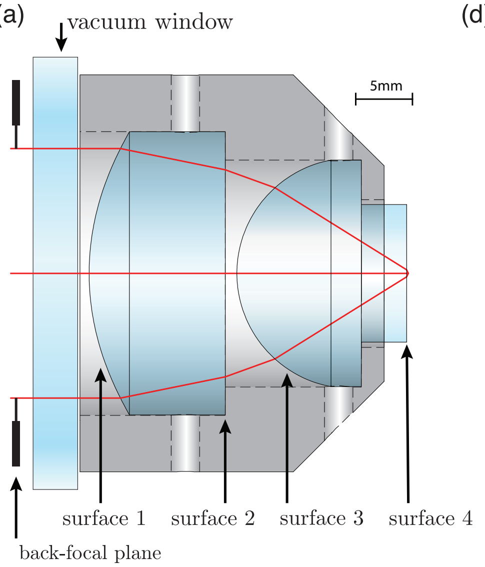


(d)

| Surface | Parameter | Value |
|---|---|---|
| surface 1 | CA | 22.5 mm |
| | 3/ | - (2) RMSi < 0.1 µm |
| | 4/ | 0.5' (0.005) |
| | 5/ | 1 × 0.04; L1 × 0.063; E0.3 |
| | MIL | S/D 10-5 |
| surface 2 | CA | 22.5 mm |
| | 3/ | 1 (0.2) |
| | 4/ | - |
| | 5/ | 1 × 0.04; L1 × 0.063; E0.3 |
| | MIL | S/D 10-5 |
| surface 3 | CA | 18.0 mm |
| | 3/ | - (1) RMSi < 0.04 µm |
| | 4/ | 0,5' |
| | 5/ | 1 × 0.04; L1 × 0.063; E0.3 |
| | MIL | S/D 10-5 |
| surface 4 | CA | 12.0 mm |
| | 3/ | RMSi < 0.0005 µm "superpolished" |
| | 4/ | - |
| | 5/ | 1 × 0.04; L1 × 0.063; E0.3 |

(b)

| Surface | Radius | Thickness | Aperture radius | Glass | Aspheric surface |
|---|---|---|---|---|---|
| surface 1 | 22.366 mm | 12.00 mm | 12.50 mm | N-SF10 | yes |
| surface 2 | inf. | 1.00 mm | 12.50 mm | AIR | no |
| surface 3 | 10.175 mm | 14.97 mm | 10.0 mm | N-SF10 | no |
| surface 4 | inf. | 150.35 µm | 10.0 mm | AIR | no |

$$z = \frac{Y^2}{R(1+\sqrt{1-(1+k)Y^2/R^2})} + A_2Y^2 + A_4Y^4 + A_6Y^6 + A_8Y^8 + A_{10}Y^{10}$$

| Surface | Conic constant (k) | $A_2$ | $A_4$ | $A_6$ | $A_8$ | $A_{10}$ |
|---|---|---|---|---|---|---|
| surface 1 | $-0.651$ | - | $1.33 \times 10^{-6}$ | $-2.90 \times 10^{-8}$ | $2.86 \times 10^{-10}$ | $-1.47 \times 10^{-12}$ |

(c)

| Surface | Type | Wavelength | AOI | Reflectivity | Polarisation |
|---|---|---|---|---|---|
| surface 1-3 | Anti Reflection | 845 nm - 898 nm | 0° - 32° | R ≤ 0.5% | p, s |
| surface 4 | Anti Reflection | 845 nm - 898 nm | 0° - 67° | R ≤ 0.5% | p, s |
| | Reflection | 1025 nm - 1070 nm | 0° - 5° | R ≥ 98% | p, s |

**Fig. 3.** Summary of the high NA (0.92) objective lens: **(a)** section drawing of the lens design consisting of an aspheric (left) and a Weierstrass-sphere solid immersion lens (right) placed in a ceramic holder (grey); also shown is the back-focal plane, which lies behind the vacuum window (5 mm-thick SF57); **(b)** surface parameters of the four lens surfaces; the aspheric surface coefficients $A_i$ of surface 1 are defined according to the surface equation $z$; **(c)** details of the surface coatings: all surfaces have an anti-reflective coating for 845 nm - 898 nm, additionally surface 4 has a high-reflective coating for 1064 nm; **(d)** surface roughness parameters according to ISO 10110: 3/ surface form tolerances, 4/ centering tolerances, 5/ surface imperfection tolerances.

## REFERENCES


1. S. U. Hwang and Y. G. Lee, "Simulation of an oil immersion objective lens: a simplified ray-optics model considering Abbe's sine condition," Opt. Express **16**, 21170 (2008).
2. J. H. Burge, C. Zhao, and S. H. Lu, "Use of the Abbe sine condition to quantify alignment aberrations in optical imaging systems," in *Proc. SPIE 7652, International Optical Design Conference 2010* (2010) p. 765219.
3. C. J. R. Sheppard and M. Gu, "Imaging by a High Aperture Optical System," J. Mod. Opt. **40**, 1631 (1993).
4. C. Obermüller and K. Karrai, "Far field characterization of diffracting circular apertures," Appl. Phys. Lett. **67**, 3408 (1995).
5. C. Obermüller, K. Karrai, G. Kolb, and G. Abstreiter, "Transmitted radiation through a subwavelength-sized tapered optical fiber tip," Ultramicroscopy **61**, 171 (1995).
6. T. Wilson, R. Juškaitis, and P. Higdon, "The imaging of dielectric point scatterers in conventional and confocal polarisation microscopes," Opt. Commun. **141**, 298 (1997)
